# Supplementary material for: Cloud-based XAI Services for Assessing Open Repository Models Under Adversarial Attacks
Source: arXiv:2401.12261 source file (2024-10-01)
Supplement: Supplementary file 1 [file appendix-attributes.tex]

\section{Specific experiments setup [TODO]}

% \section{Practical Approaches to Evaluating Quality Attributes of Vision Models under Adversarial Conditions}

\textcolor{red}{Followed by the functionality overview, this section justifies in detail the practical approaches to achieve the evaluation}

In this section, we list general XAI-based quality attributes for vision models that need to be evaluated under adversarial attacks. Then, we discuss the complex factors that exist in evaluations.

\subsection{Computational Efficiency}

A practical approach to estimating computational resources begins with measuring the utilization of GPUs \cite{runtime-based}. 
CUDA-enabled GPUs are integral to AI applications due to the following two key factors \cite{runtime-based}: (1) The wide support they receive across major machine learning frameworks, such as TensorFlow \cite{TensorFlow} and PyTorch \cite{PyTorch}. (2) Both cloud platforms and local setup options facilitate the accessibility of GPUs. 
We refer to the approach and provide the computational runtime measurements. 

\subsection{Model Performance}
Evaluating model quality attributes fundamentally requires an analysis of general performance metrics. 
we include precision and recall metrics \cite{presicionrecall}. These metrics offer insights into the accuracy of positive predictions and the model’s capacity to identify all positive instances, respectively. The F1 Score \cite{presicionrecall}, as the harmonic mean of precision and recall, is also utilized, serving as a critical balanced metric in situations where trade-offs are necessary.

To assess a model's discriminative ability between classes, we employ the AUC-ROC \cite{ROC}. Particularly in a multi-class context, this is adapted through micro-averaging, which aggregates outcomes across all classes to yield a comprehensive measure of the model's overall performance. The Area Under the Curve emerges as a key metric in this evaluation.

\subsection{Model Robustness}
\label{sec:RobustnessMetric}
To test the robustness of the selected model, we add the corruptions are algorithmically generated from three general categories \cite{imagenetC}: Gaussian Noise, Defocus Blur, and Pixelate. These corruptions are applied to the evaluation dataset, resulting in a set of perturbed images for robustness testing.
We apply three levels of severity for each corruption type.
With the levels increasing, we can test and observe the model's performance decreases.

The impact of image corruption on AI model performance varies with these types. Gaussian Noise tests a model's capacity to discern signal from noise, a critical factor in accurately identifying details. Defocus Blur alters spatial information, impacting models that rely on precise edge and texture recognition. Pixelation test models by reducing resolution. These corruptions challenge the vision model's ability to maintain accuracy with minor perturbed visual inputs, thereby evaluating its robustness in real-world conditions where such image quality issues are common.
Systematically applying these corruptions allows AI system developers and researchers to identify the weaknesses among the published open-source models.
For instance, models that perform well on clean images but poorly on corrupted ones may be overfitting to high-resolution data and lacking in generalization capabilities. This evaluation suggests a more resilient model architecture for real-world applications.

As a quantifiable metric, Kolmogorov-Smirnov (K-S) statistic \cite{KolmogorovSmirnov} is designed to determine if two samples are drawn from the same distribution \cite{KolmogorovSmirnov}. This method focuses on comparing the distribution of the model's confidence outputs across large datasets. It assesses the impact of adversarial perturbations on the output distribution of AI models.

The implementation steps for the modified K-S statistic in evaluating AI model robustness are as follows:
\begin{enumerate}
    \item For the original dataset, collect the maximum softmax probability for each sample.
    \item Repeat the process for the attacked (or perturbed) dataset.
    \item Form two distributions: one from the original dataset's maximum probabilities and one from the attacked dataset's.
    \item Calculate the K-S statistic to quantify the disparity between these two distributions.
\end{enumerate}

The K-S statistic, in this context, is computed as:
\begin{equation}
    D_{KS} = \max_{x} | F_{\text{original}}(x) - F_{\text{attacked}}(x) |
\end{equation}
where \( F_{\text{original}}(x) \) and \( F_{\text{attacked}}(x) \) are the distributions of the maximum confidence scores for the original and attacked datasets.

A higher value of \( D_{KS} \) indicates a significant shift in the model's confidence distribution when exposed to perturbations, suggesting reduced robustness. Conversely, a lower \( D_{KS} \) value suggests that the model maintains its confidence levels, indicating robustness against such adversarial attacks.

The K-S statistic is advantageous as it provides a non-parametric way to assess the difference in model outputs due to perturbations, without assuming any specific distribution of these outputs. This makes it a versatile tool for robustness evaluation, capable of handling various types of model architectures and output distributions.

This modified approach of using K-S statistic provides a practical and efficient means to assess model robustness in large-scale scenarios, enabling a comprehensive understanding of how adversarial perturbations impact the model's confidence across the entire dataset.

\subsection{XAI-based Quality Attributes}
\textcolor{red}{Attribution selection, introduce Saliency methods}
Saliency methods, often used in image classification, assess pixel importance for the output and create visual maps. It is important to note that in our scenarios, where sensitive labels are not defined in the ImageNet \cite{ImageNet}, fairness is not included as a metric. However, when the framework is applied to tabular data models, fairness can be customized as an attribute with user-defined sensitive labels \cite{alikhademi2021can}.

Gradient-based XAI methods are initially designed for CNN-based models. Recent work has extended their application to vision transformers in the sensitive medical field \cite{shome2021covid,sobahi2022explainable}, aiming to offer explanations for these transformer-based models. However, whether these XAI techniques perform as effectively for transformer-based models as for CNN-based models remains an open research question. 

%Faithfulness can be evaluated by observing the impact of incremental feature modifications on model predictions, while stability is assessed through the consistency of explanations against minor perturbations in the input. This intrinsic measurability makes both metrics particularly appealing for our study, ensuring our evaluation framework is broadly applicable and not constrained by the availability of specialized external annotations or datasets.

% We prioritize faithfulness and stability to ensure a robust and universally applicable framework for evaluating XAI techniques. This choice is not only pragmatic, given the common constraints of existing datasets, but also strategic, enabling us to focus on those metrics that provide the most direct insight into the efficacy of explanations across a wide array of models and scenarios without the need for additional, often unavailable, data preparation.

Here, we specify the steps to evaluate the vision model's saliency map faithfulness. We overlay the original images with their corresponding saliency maps and then re-input them into the model. 
This step assesses whether these saliency-highlighted areas dictate the model's classification predictions. If the model's prediction scores change minimally upon this intervention, it suggests that these areas indeed lead to the exact predictions. 
Conversely, significant shifts in prediction scores would indicate a misalignment between the saliency maps and the actual decision-driving features of the model.

The steps of applying a saliency map explanation to mask an image are as follows:
\begin{enumerate}
    \item Normalize the grayscale mask.
    \item Extend the mask dimensions to match those of the image.
    \item Apply the mask to the original image.
\end{enumerate}

The grayscale mask, denoted by \( M \), is a two-dimensional array of values representing the intensity or weight to be applied to each pixel of the image. Specifically, let \( M \in \mathbb{R}^{h' \times w'} \) represent this mask, where \( h' \) and \( w' \) are its height and width, respectively.

The mask is typically normalized to ensure that its values are within a standard range. This normalization process adjusts the values of \( M \) to be between 0 and 1, and is achieved using the formula:

\begin{equation}
M_{\text{norm}} = \frac{M - \min(M)}{\max(M) - \min(M)}
\end{equation}

% \[ M_{\text{norm}} = \frac{M - \min(M)}{\max(M) - \min(M)} \]
Here, \( \min(M) \) and \( \max(M) \) represent the minimum and maximum values found within the mask \( M \). The normalization ensures that the mask can be combined with the image data.

The normalized mask \( M_{\text{norm}} \) is extended to three dimensions to match the RGB channels of the image:

\begin{equation}
M_{3D} = \text{repeat}(M_{\text{norm}}, 3, \text{axis} = 2)
\end{equation}

Here, \( M_{3D} \in \mathbb{R}^{h \times w \times 3} \).

The masked image \( I_{\text{masked}} \) is then computed as the element-wise product of the image and the extended mask:

\begin{equation}
I_{\text{masked}} = I \cdot M_{3D}
\end{equation}

where \( \cdot \) denotes element-wise multiplication.

Finally, the explanation utility is a metric that measures how much a model's predictions change when we compare an original image with a masked version. It is calculated by one minus the overall difference in the model's prediction for these two images. A smaller score drop indicates a high explanation utility, meaning the model can still make reliable predictions even with incomplete information. 
%Evaluations of the XAI methods and the combination of models with explanation utility are essential to developing trustworthy AI systems.

% Overall, this study provides a scenario that evaluates the CAM series XAI methods \cite{Grad-cam,Grad-cam++,xgradcam,layercam} for the emerging Transformer-based models. The scenario evaluates if their combination integration is effective in the AI systems software.  
% %\cite{Grad-cam,Grad-cam++，HiResCAM,xgradcam,layercam} 

\subsection{Explanation Resilience}
\label{sec:explanation-resilience}

% To evaluate the resilience of the XAI methods to adversarial conditions, we introduced adversarial perturbations to the input data and observed the variations in explanation utility. The evaluation is based on the metric of explanation utility.

% We quantified the explanation resilience as \(1-x\), where \(x\) represents the rate of change in explanation utility post-perturbation. This approach allows us to assess the XAI methods in adversarial scenarios. 

To evaluate the resilience of the XAI methods to adversarial conditions, we introduced adversarial perturbations to the input data and observed the variations in explanation utility. 
The evaluation is based on the metric of explanation utility. 
We compute the overall explanation utility under original data and adversarial perturbed data. The difference in ratio can be calculated.

Considering adversarial perturbations increases the value of explanation utility, which makes the value larger than one. 
We present the combined equation to normalize the change.

The normalized resilience is quantified by the following formula:
\begin{equation}
\text{Resilience} = (O) \times  (1 - P) 
\end{equation}
where \(O\) and \(P\) represent the value of the original explanation utility and the change in the explanation utility, respectively. The term \(1 - P\) reflects the model's ability to maintain its explanation utility under adversarial conditions, with a higher value indicating greater resilience. This formulation allows for an assessment of how well the XAI methods withstand adversarial scenarios, taking into account both their performance under perturbation and their baseline effectiveness.

Overall, the evaluation of AI systems, particularly under adversarial conditions, involves a complex interplay of multiple factors. This complexity stems from the diverse AI models, the wide array of adversarial perturbation methods, and the evolving spectrum of XAI techniques. 

Given these multi-faceted challenges, we present a conceptual framework for quality attribute evaluations. The framework provides a structured and systematic process to evaluate AI systems, taking into account the various dimensions of model performance, robustness, and explanation utility. It enables AI practitioners to navigate the intricacies of different model architectures, adversarial methods, and XAI techniques, providing a comprehensive understanding of the AI-based system's capabilities and limitations.
